# Supplementary material for: Scattering Loss in Precision Metrology due to Mirror Roughness
Source: arXiv:2201.05640 source file (2022-01-14)
Supplement: Supplementary file 1 [file Appendix.tex]

\appendix

\section{On-Resonance Reflectivity for Cavity Loss Estimation}
\label{app:dc-method}

Here we derive the equations that let us extract round-trip loss estimates from reflected power measurements. This is explicitly done for the case of a linear two-mirror cavity, but the extension to the case of multiple mirrors is straightforward. We start with the conservation of energy upon reflection from a single mirror, given by
\begin{equation}
	R_i+T_i+\mathcal{L}_i = 1,
	\label{eq:TR_sum}
\end{equation}
where $R_i$ is the reflectance, $T_i$ is the transmittance, and $\mathcal{L}_i$ is the optical loss of mirror $i$ for light impinging on the HR-coated side, which is assumed facing the inside of the cavity. Bulk scatter and absorption in the mirror substrate, as well as the residual reflection from the AR-coating, introduce additional losses for reflections seen from the AR-coated side. Moreover, layer defects and surface contamination can effect loss differences on either side of the HR coating. However, in the comparative approach of the DC-method, these discrepancies become optical losses of the beam path outside the cavity and affect both reflected power measurements equally. They cancel in combination, which allows us to consider \Cref{eq:TR_sum} valid on both sides of the mirror.

In this case, $\mathcal{L}_i$ represents each mirror's contribution to the cavity round-trip loss, which is a combination of HR coating absorption and scatter loss from the mismatch between mirror surface and cavity mode wavefront. The round-trip loss of the two-mirror cavity is then
\begin{equation}
	\mathcal{L} = \mathcal{L}_1+\mathcal{L}_2,
	\label{eq:loss_sum}
\end{equation}
where we use the index $1$ for the input mirror (ITM) and the index $2$ for the back mirror (ETM). We further define the transmission coefficients
\begin{equation}
	 t_i = \sqrt{T_i}
	 \label{eq:ti_Ti}
\end{equation}
and the reflection coefficients
\begin{equation}
	r_i=\sqrt{R_i}=\sqrt{1-T_i-\mathcal{L}_i}
	\label{eq:ri_Ri}
\end{equation}
for the electromagnetic field. On resonance, the compound reflection coefficient of a linear optical cavity formed by mirrors 1 and 2 is
\begin{equation}
	r_\mathrm{r} = \frac{r_1-r_2\left(r_1{}^2+t_1{}^2\right)}{1-r_1r_2}.
 \end{equation}
%This expression is positive for under-coupled cavities ($T_1<\mathcal{L}+T_2$), negative for over-coupled cavities ($T_1>\mathcal{L}+T_2$), indicating a phase-flip upon reflection, and zero in the impedance-matched case ($T_1=\mathcal{L}+T_2$).

To evaluate $\mathcal{L}$, we compare the reflection of an incoming laser beam in two cases. First, for prompt reflections off mirror 1 the reflectance is
\begin{equation}
	R_m=1-T_1-\mathcal{L}_1.
	\label{eq:R_m}
\end{equation}
It is important to note that an aligned but off-resonant optical cavity behind mirror 1 results in a boosted compound reflection compared to the single mirror case. It is thus necessary to misalign the cavity optics or otherwise block the intra-cavity beam path to measure \Cref{eq:R_m}. 

In the resonant case with perfect overlap of incident beam and cavity eigenmode, the cavity reflectance is
\begin{equation}
	R_r=\left|\frac{\sqrt{1-T_1-\mathcal{L}_1}-\sqrt{1-T_2-\mathcal{L}_2}\left(1-\mathcal{L}_1\right)}{1-\sqrt{(1-T_1-\mathcal{L}_1)(1-T_2-\mathcal{L}_2)}}\right|^2.
\end{equation}
To account for mode mismatch, we introduce the visibility factor $\eta$, which quantifies the fraction of incident optical power in the fundamental cavity mode. Additionally, we use a factor $\gamma$ to describe the fraction of optical power in the resonant carrier. The remaining power fraction $1-\gamma$ is shifted to sidebands by phase modulation of the carrier to generate various error signals for interferometer state control. Laser frequency sweeps can be used to measure both $\eta$ and $\gamma$ by observing the transmitted cavity power spectrum of carrier and sidebands in fundamental and higher order modes. Only the fraction $\eta\gamma P_0$ of the incident power $P_0$ interacts with the cavity during the DC measurement. The reflected power on resonance becomes
\begin{equation}
P_r=(1-\eta\gamma)P_0+\eta\gamma R_rP_0,
\label{eq:P_r}
\end{equation}
while in the misaligned case the reflected power remains
\begin{equation}
P_m=R_mP_0.
\label{eq:P_m}
\end{equation}
Dividing \Cref{eq:P_r} by \Cref{eq:P_m} yields
\begin{equation}
\frac{P_r}{P_m}=\frac{1-\eta\gamma(1-R_r)}{R_m}.
\label{eq:P_div}
\end{equation}
Given measurements for $T_1$, $T_2$, $\eta$, and $\gamma$, we can infer values of $\mathcal{L}_1$ and $\mathcal{L}_2$ which result in the observed power levels. Assuming equal losses $\mathcal{L}_1=\mathcal{L}_2=\mathcal{L}/2$, this turns into a direct measurement of $\mathcal{L}$. Since this is not a phase-sensitive measurement, there will always be two solutions (one for the over-coupled case $T_1>T_2+\mathcal{L}$ and one for the under-coupled case $T_1<T_2+\mathcal{L}$). The arm cavities of GWDs and their prototypes are highly over-coupled, meaning we can safely assume that the correct solution is the smaller loss value.

The advantage of this method is that in the fractional comparison of $P_r$ and $P_m$, the comparatively large absolute uncertainty in $T_1$ compared to expected values of $\mathcal{L}$ does not completely dominate the uncertainty in loss estimates. To show this explicitly, we approximate $r_i$ for an HR mirror as
\begin{equation}
	r_i\approx1-\frac{T_i}{2}-\frac{\mathcal{L}_i}{2}-\frac{T_i{}^2}{8}+\mathcal{O}\left(T_i\mathcal{L}_i,\mathcal{L}_i{}^2\right).
	\label{eq:r_approx}
\end{equation}
In typical arm cavities of GW detectors, including the 40\,m prototype, $T_1$ is of order $1\,\%$, while the expected per-mirror loss is 10-100\,ppm. This results in a similar magnitude of the $\mathcal{O}(T_1{}^2)$ term in the equation and its preceding $\mathcal{L}_i$ term, making it necessary to carry the term quadratic in $T_1$ in the derivation. The relative magnitude of the error introduced by \Cref{eq:r_approx} is at most of order $10^{-5}$ for the above parameters, and of order $10^{-9}$ for an ETM-like configuration.

On resonance, the compound reflection coefficient of a linear optical cavity formed by two mirrors with labels 1 and 2 is
\begin{equation}
	r_\mathrm{r} = \frac{r_1-r_2\left(r_1{}^2+t_1{}^2\right)}{1-r_1r_2}.
 \end{equation}
Using \Cref{eq:ti_Ti}, \Cref{eq:ri_Ri}, and \Cref{eq:r_approx} we can approximate this as
\begin{equation}
	r_\mathrm{r}\approx1-2\frac{T_1+\frac{T_1{}^2}{4}}{T_1+\frac{T_1{}^2}{4}+T_2+\mathcal{L}},
\end{equation}
which contains all terms with magnitude large or similar to the leading loss terms. The power reflection $R_\mathrm{r} = \left|r_\mathrm{r}{}\right|^2$ of the resonant cavity is accordingly given by
\begin{equation}
	R_\mathrm{r} = \left|1-4\frac{\left(T_1+\frac{T_1{}^2}{4}\right)\left(1-\frac{T_1+\frac{T_1{}^2}{4}}{T_1+\frac{T_1{}^2}{4}+T_2+\mathcal{L}}\right)}{T_1+\frac{T_1{}^2}{4}+T_2+\mathcal{L}}\right|.
\end{equation}
For strongly overcoupled cavities this can be simplified to 
\begin{equation}
	R_\mathrm{r} \approx \left|1-4\frac{\mathcal{L}+T_2}{T_1+\frac{T_1{}^2}{4}+T_2+\mathcal{L}}\right|.
\end{equation}
With $T_1\gg T_2,\mathcal{L}$, the second term in this expression is small, resulting in values of $R_r$ close to unity.

We now compare the reflection off the ITM in two cases. First, the pure ITM reflection $P_1$ when either the ETM is misaligned or the optical path in the cavity is otherwise blocked is
\begin{equation}
	P_1=R_1P_0=(1-T_1-\mathcal{L}_1)P_0.
%	\label{eq:P_1}
\end{equation}
On the other hand, in the resonant case with optimal beam alignment the resonant cavity reflection $P_r$ is
\begin{equation}
	P_r=R_rP_0=\left(1-4\frac{\mathcal{L}+T_2}{T_1}\right)P_0.
\end{equation}
%This is a well-known relationship, which shows that there is not cavity reflection when the cavity is impedance matched, $T_1=T_2+\mathcal{L}$.

estimate $\mathcal{L}$ by dividing \Cref{eq:P_r} by \Cref{eq:P_1}. In \Cref{fig:refl-loss} we plot this ratio $P_r/P_m$ as a function of round-trip arm loss for the nominal 40\,m prototype parameters, which are listed along with their uncertainties in \Cref{tab:40m-parameters}. In the calculation $P_r/P_m$ it was assumed that $\mathcal{L}_1=\mathcal{L}/2$.
\begin{equation}
P_r = (1-\eta\gamma)P_0+\eta\gamma R_rP_0\approx \left(1-4\eta\gamma\frac{\mathcal{L}+T_2}{T_1}\right)P_0.
%\label{eq:P_r}
\end{equation}

In the aligned, resonant case we have to account for mode-mismatch and the reduced visibility $\eta$ (quantified as fraction of optical power in the fundamental mode): a fraction $1-\eta$ of the incident light does not contribute any cavity effects. We obtain
\begin{equation}
P_r{}'=(1-\eta)P_0+\eta R_rP_0\approx\left(1-4\eta\frac{\mathcal{L}+T_2}{T_1}\right)P_0
% (1-\eta)P_{in}+\eta\left(1-4\frac{\mathcal{L}+T_2}{T_1}\right)P_{in}
\end{equation}
This also needs to be corrected for the power content in phase modulation sidebands, which are used to obtain the various cavity error and alignment signals with the PDH technique. The series expansion of the electric field for pure phase modulation with modulation depth $\beta$ reads
\begin{equation}
E=E_0\mathrm{e}^{i\omega t}\mathrm{e}^{i\beta\Omega t}=E_0\mathrm{e}^{i\omega t}\sum_{n=-\infty}^{\infty}\limits J_n(\beta)\mathrm{e}^{i\Omega t}%=E_0\mathrm{e}^{i\omega t}J_0(\beta)+\mathrm{sideband~terms}
\end{equation}
The fraction of power remaining in the carrier for each phase modulation with modulation depth $\beta_i$ is $J_0{}^2(\beta_i)$. For $N$ modulations, we define the fraction $\gamma$ of power remaining in the carrier as
\begin{equation}\\
\gamma=\prod_{i=1}^N\limits J_0(\beta_i)^2\stackrel{N=2}{=}J_0(\beta_1)^2\times J_0(\beta_2)^2.
\end{equation}
The phase modulation transfers a fraction $1-\gamma$ of light power from the carrier to sidebands. Similar to the junk light content $1-\eta$, this portion does not resonate in the arm cavities. We can thus write the compound correction to $P_r$ as
%\begin{equation}
%P_0 = \textcolor{red}{\underbrace{(1-\eta)P_0}_\mathrm{junk light}+\underbrace{\eta(1-\gamma)P_{in}}_\mathrm{sidebands}}\textcolor{blue}{+\underbrace{\eta\gamma P_{in}}_\mathrm{carrier}}=\textcolor{red}{(1-\eta\gamma)P_{in}}+\textcolor{blue}{\eta\gamma P_0}.
%\end{equation}
\begin{equation}
P_r = (1-\eta\gamma)P_0+\eta\gamma R_rP_0\approx \left(1-4\eta\gamma\frac{\mathcal{L}+T_2}{T_1}\right)P_0.
%\label{eq:P_r}
\end{equation}
Given measurements for the quantities $T_1$, $T_2$, $\eta$, and $\gamma$, we can estimate $\mathcal{L}$ by dividing \Cref{eq:P_r} by \Cref{eq:P_1}. In \Cref{fig:refl-loss} we plot this ratio $P_r/P_m$ as a function of round-trip arm loss for the nominal 40m prototype parameters, which are listed along with their uncertainties in \Cref{tab:40m-parameters}. In the calculation $P_r/P_m$ it was assumed that $\mathcal{L}_1=\mathcal{L}/2$.
